# Supplementary material for: Semantic Example Guided Image-to-Image Translation
Source: arXiv:1909.13028 source file (2019-10-04)
Supplement: Supplementary file 1 [file appendix.tex]

\subsection*{Implementation Details}
\textbf{General settings} Our major network contains an encoder for the reference and the input image, two decoders for the target image and the segmentation. We use 6 combined convolution blocks with Relu activation layer and batch normalization layers for the encoder and add 5 non-local layers in total, two of them are at the bottleneck while the other three are in the decoder for the target image. Residual blocks with two 3x3 convolutional blocks are used in between the first two non-local layers. To avoid checkerboard effects mentioned in the previous work\cite{checkerboard}, we use a combination of up-sample and convolution to replace deconvolution layers in our decoders. Instead of using batch normalization, we adopt spectral normalization\cite{sn} as training stabilization techniques in our discriminator to achieve better image quality. We adopted different learning rate for the generator ($2e^{-4}$) and discriminator ($1.3e^{-5}$), and for weights of different objectives are: $w_1=w_4=100.0, w_2=5e^{-6},w_4=1.0, w_5=w_6=10.0$, parameters are kept as the same for all the experiments in this work unless specific modification is mentioned later. For datasets containing more than 50K images(sketch2shoes\cite{edge1}, sketch2bags\cite{edge2}, celebA\cite{celeba}), we use a batch size of 5 and around 20 epochs to achieve satisfactory and stable results. With two NVIDIA 2080Ti GPUs, it takes about 20 hours to finish the training. For smaller datasets, 12-epoch with training time around 10 hours should be enough.\par
\textbf{Network Structure} Our model consists of two parts, the input image and the reference are sent to the preprocess network (semantic match), the output of which then is used as input of the major network. The major network starts with an encoder, and we add two non-local layers after the bottleneck layer, which are followed by a 3x3 residual block respectively. We adopt two decoders to generate different output images. We also adopt the U-net structure\cite{unet} for the major decoder.\par
\begin{figure}[!ht]
\includegraphics[width=\textwidth]{fig/network_structure.png}
\centering
\caption{\small{Network pipeline}}
\label{fig:network}
\end{figure}
\textbf{Training techniques and tricks} Several training tricks are used in the training process to improve the performance as well as robustness. (1) We add an mask to indicate the valid pixels of the w(x, r), it is mentioned in \cite{inpainting} that concating image with invalid pixels (white space) in the $\mathcal{W}(x, r)$ will cause blurry outputs with skewed boundary around those white space. Therefore we add a binary mask to indicate the locations of the valid pixels in $\mathcal{W}(x, r)$. (2) Label flipping, in our experiments for all the dataset we train two batches on the regular label and then train one batches on the flipped label that $real:0, fake:1$. (3) We also add noise images in the training process that using some random shuffled images as $\mathcal{W}(x,y)$ with $5\%$ probability to improve the robustness of the network.

\subsection*{Ablation Study}
We conduct ablation experiments to demonstrate that the non-local block and the multi-task framework have an essential contribution to improve the output in terms of color propagation as well as the generation of complete object boundary. We notice that color cannot be propagated properly in the results generated without the non-local layers. While without the multi-task framework that can generate attention mask, the output disposes of artifacts around the edge of objects. We also found those artifacts in prior works\cite{pix2pix,munit}, and it can be eliminated by generating the attention mask as auxiliary information. We show some ablation study results in Fig.\ref{fig:abl} 
\begin{figure}[!ht]
\centering
\begin{subfigure}{1.5cm}
\includegraphics[trim=0cm 0cm 0cm 0cm,clip=true,width=1.5cm]{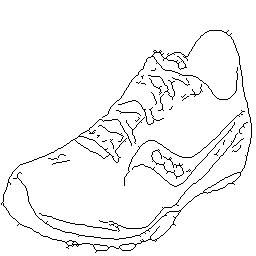}
\end{subfigure}
\begin{subfigure}{1.5cm}
\includegraphics[trim=0cm 0cm 0cm 0cm,clip=true,width=1.5cm]{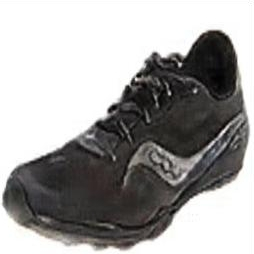}
\end{subfigure}
\begin{subfigure}{1.5cm}
\includegraphics[trim=0cm 0cm 0cm 0cm,clip=true,width=1.5cm]{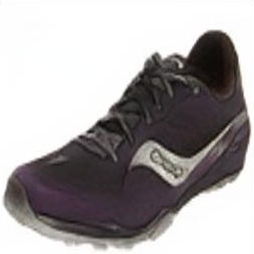}
\end{subfigure}
\begin{subfigure}{1.6cm}
\includegraphics[trim=0cm 0cm 0cm 0cm,clip=true,width=1.5cm]{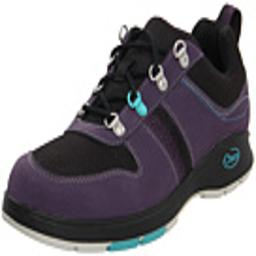}
\end{subfigure}\vline
\begin{subfigure}{1.5cm}
\includegraphics[trim=0cm 0cm 0cm 0cm,clip=true,width=1.5cm]{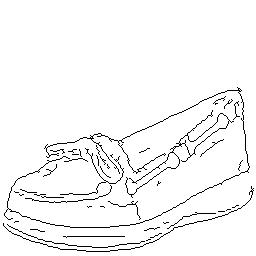}
\end{subfigure}
\begin{subfigure}{1.5cm}
\includegraphics[trim=0cm 0cm 0cm 0cm,clip=true,width=1.5cm]{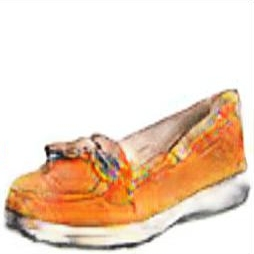}
\end{subfigure}
\begin{subfigure}{1.5cm}
\includegraphics[trim=0cm 0cm 0cm 0cm,clip=true,width=1.5cm]{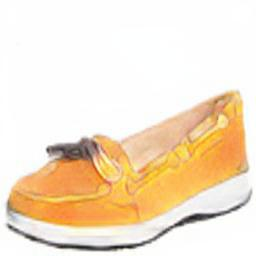}
\end{subfigure}
\begin{subfigure}{1.5cm}
\includegraphics[trim=0cm 0cm 0cm 0cm,clip=true,width=1.5cm]{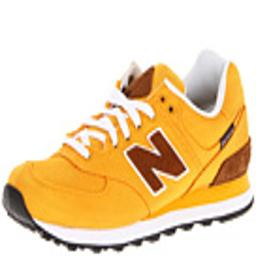}
\end{subfigure}
\begin{subfigure}{1.5cm}
\includegraphics[trim=0cm 0cm 0cm 0cm,clip=true,width=1.5cm]{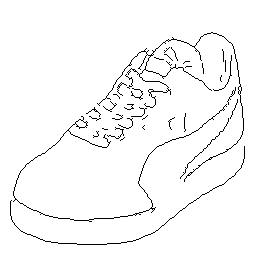}\caption*{\small{Input}}
\end{subfigure}
\begin{subfigure}{1.5cm}
\includegraphics[trim=0cm 0cm 0cm 0cm,clip=true,width=1.5cm]{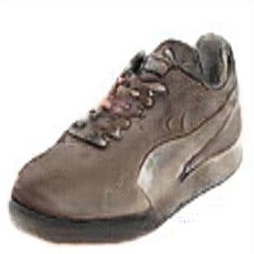}\caption*{\small{w/o NL}}
\end{subfigure}
\begin{subfigure}{1.5cm}
\includegraphics[trim=0cm 0cm 0cm 0cm,clip=true,width=1.5cm]{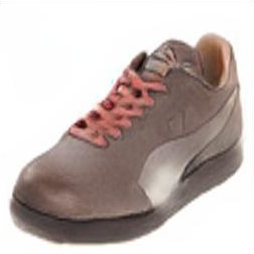}\caption*{\small{w/ NL}}
\end{subfigure}
\begin{subfigure}{1.6cm}
\includegraphics[trim=0cm 0cm 0cm 0cm,clip=true,width=1.5cm]{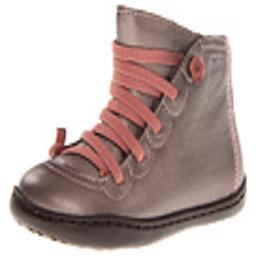}\caption*{\small{Ref}}
\end{subfigure}\vline
\begin{subfigure}{1.5cm}
\includegraphics[trim=0cm 0cm 0cm 0cm,clip=true,width=1.5cm]{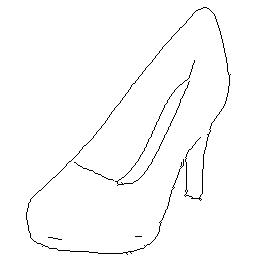}\caption*{\small{Input}}
\end{subfigure}
\begin{subfigure}{1.5cm}
\includegraphics[trim=0cm 0cm 0cm 0cm,clip=true,width=1.5cm]{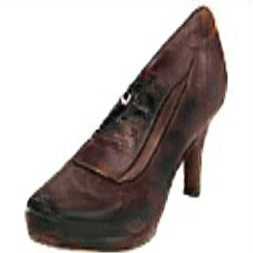}\caption*{\small{w/o MT}}
\end{subfigure}
\begin{subfigure}{1.5cm}
\includegraphics[trim=0cm 0cm 0cm 0cm,clip=true,width=1.5cm]{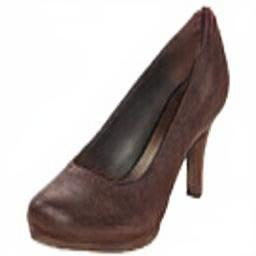}\caption*{\small{w/ MT}}
\end{subfigure}
\begin{subfigure}{1.5cm}
\includegraphics[trim=0cm 0cm 0cm 0cm,clip=true,width=1.5cm]{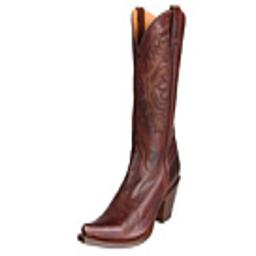}\caption*{\small{Ref}}
\end{subfigure}
\caption{\small{NL indicates the non-local layers while MT represents the multi-task architecture. It is shown that w/o NL, colors cannot be propagated properly, and the model tends to paste general color(black, gray) at those locations; while w/o the multi-task component, the model cannot focus on generating data within a specific range, which will cause artifacts and blending color shown in the second column on the right side.}}
\label{fig:abl}
\end{figure}
\subsection*{More Results}
 We also improve the sketch generation method by combining the Hed\cite{hed} with sketch simplification\cite{sketchimprove}, which can increase the quality of outputs. We presents the results with improved sketches as input on edge2handbags and anime dataset, but we use the standard sketch for all the comparison with other models mentioned in this work to keep the equity. More results generated with the refined sketches are shown in Fig.\ref{fig:morebags}-\ref{fig:moreshoes}.\par
\begin{figure}[!ht]
    \centering
    \includegraphics[width=1.6cm]{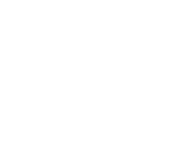}
    \includegraphics[width=1.6cm]{fig/white.png}
    \begin{subfigure}{1.6cm}
    \includegraphics[trim=0cm 0cm 0cm 0cm,clip=true,width=1.6cm]{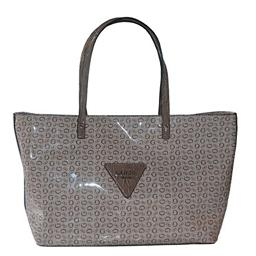}\vspace{-0.1cm}\caption*{\small{Ref 1}}
    \end{subfigure}
    \begin{subfigure}{1.6cm}
    \includegraphics[trim=0cm 0cm 0cm 0cm,clip=true,width=1.6cm]{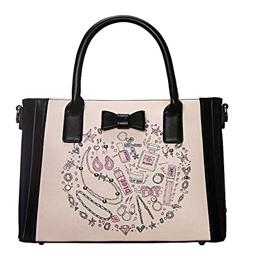}\vspace{-0.1cm}\caption*{\small{Ref 2}}
    \end{subfigure}
    \begin{subfigure}{1.6cm}
    \includegraphics[trim=0cm 0cm 0cm 0cm,clip=true,width=1.6cm]{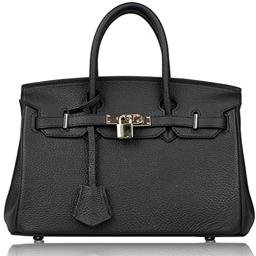}\vspace{-0.1cm}\caption*{\small{Ref 3}}
    \end{subfigure}
    \begin{subfigure}{1.6cm}
    \includegraphics[trim=0cm 0cm 0cm 0cm,clip=true,width=1.6cm]{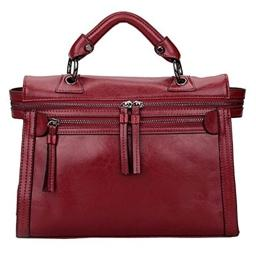}\vspace{-0.1cm}\caption*{\small{Ref 4}}
    \end{subfigure}
    \begin{subfigure}{1.6cm}
    \includegraphics[trim=0cm 0cm 0cm 0cm,clip=true,width=1.6cm]{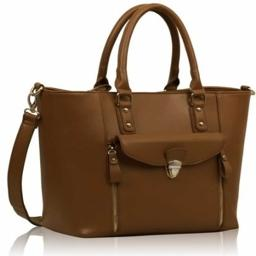}\vspace{-0.1cm}\caption*{\small{Ref 5}}
    \end{subfigure}
    \begin{subfigure}{1.6cm}
    \includegraphics[trim=0cm 0cm 0cm 0cm,clip=true,width=1.6cm]{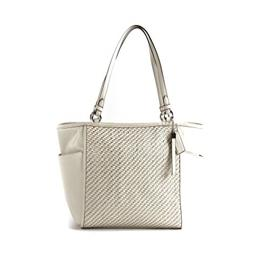}\vspace{-0.1cm}\caption*{\small{Ref 6}}
    \end{subfigure}
    
    \includegraphics[width=1.6cm]{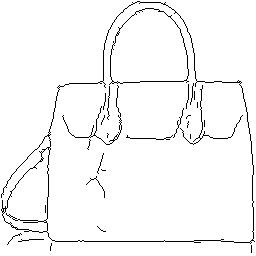}
    \includegraphics[width=1.6cm]{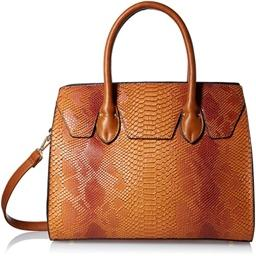}
    \includegraphics[trim=0cm 0cm 0cm 0cm,clip=true,width=1.6cm]{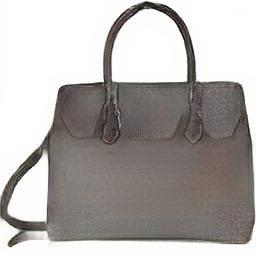}
    \includegraphics[trim=0cm 0cm 0cm 0cm,clip=true,width=1.6cm]{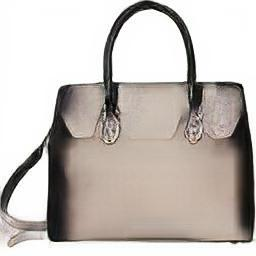}
    \includegraphics[trim=0cm 0cm 0cm 0cm,clip=true,width=1.6cm]{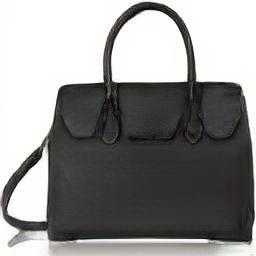}
    \includegraphics[trim=0cm 0cm 0cm 0cm,clip=true,width=1.6cm]{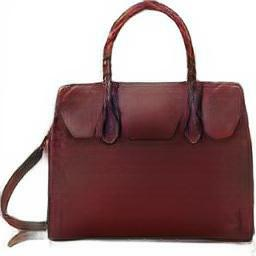}
    \includegraphics[trim=0cm 0cm 0cm 0cm,clip=true,width=1.6cm]{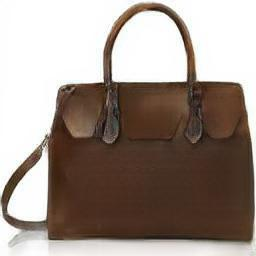}
    \includegraphics[trim=0cm 0cm 0cm 0cm,clip=true,width=1.6cm]{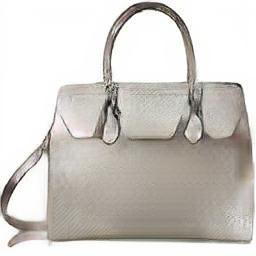}
    
    \begin{subfigure}{1.6cm}
    \includegraphics[trim=1cm 0cm 1cm 0cm,clip=true,width=1.6cm]{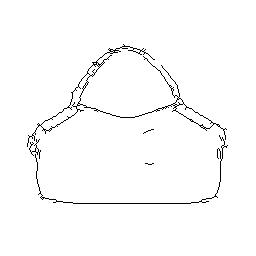}\vspace{-0.1cm}\caption*{\small{Input}}
    \end{subfigure}
    \begin{subfigure}{1.6cm}
    \includegraphics[trim=1cm 0cm 1cm 0cm,clip=true,width=1.6cm]{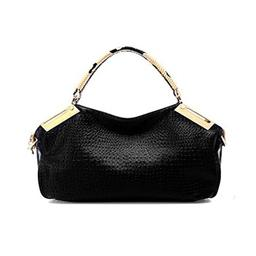}\vspace{-0.1cm}\caption*{\small{GT}}
    \end{subfigure}
    \begin{subfigure}{1.6cm}
    \includegraphics[trim=1cm 0cm 1cm 0cm,clip=true,width=1.6cm]{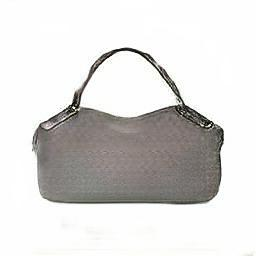}\vspace{-0.1cm}\caption*{\small{Result 1}}
    \end{subfigure}
    \begin{subfigure}{1.6cm}
    \includegraphics[trim=1cm 0cm 1cm 0cm,clip=true,width=1.6cm]{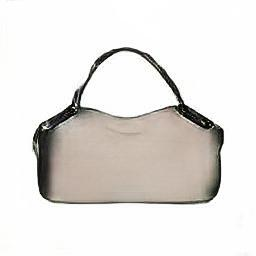}\vspace{-0.1cm}\caption*{\small{Result 2}}
    \end{subfigure}
    \begin{subfigure}{1.6cm}
    \includegraphics[trim=1cm 0cm 1cm 0cm,clip=true,width=1.6cm]{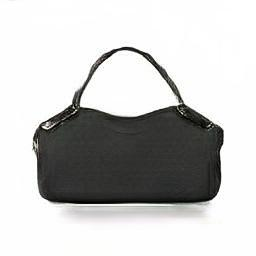}\vspace{-0.1cm}\caption*{\small{Result 3}}
    \end{subfigure}
    \begin{subfigure}{1.6cm}
    \includegraphics[trim=1cm 0cm 1cm 0cm,clip=true,width=1.6cm]{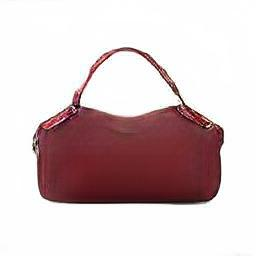}\vspace{-0.1cm}\caption*{\small{Result 4}}
    \end{subfigure}
    \begin{subfigure}{1.6cm}
    \includegraphics[trim=1cm 0cm 1cm 0cm,clip=true,width=1.6cm]{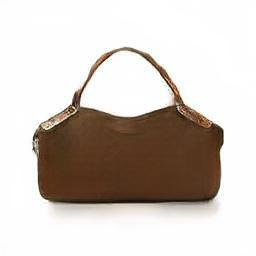}\vspace{-0.1cm}\caption*{\small{Result 5}}
    \end{subfigure}
    \begin{subfigure}{1.6cm}
    \includegraphics[trim=1cm 0cm 1cm 0cm,clip=true,width=1.6cm]{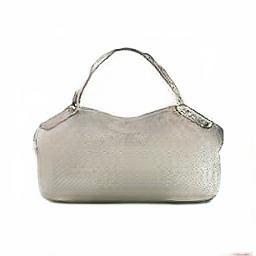}\vspace{-0.1cm}\caption*{\small{Result 6}}
    \end{subfigure}
    \caption{Results in bag dataset with the refined sketches}
    \label{fig:morebags}
\end{figure}

\begin{figure}[!ht]
    \centering
    \includegraphics[width=1.6cm]{fig/white.png}
    \includegraphics[width=1.6cm]{fig/white.png}
    \begin{subfigure}{1.6cm}
    \includegraphics[trim=0cm 0cm 0cm 0cm,clip=true,width=1.6cm]{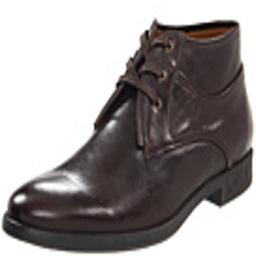}\vspace{-0.1cm}\caption*{\small{Ref 1}}
    \end{subfigure}
    \begin{subfigure}{1.6cm}
    \includegraphics[trim=0cm 0cm 0cm 0cm,clip=true,width=1.6cm]{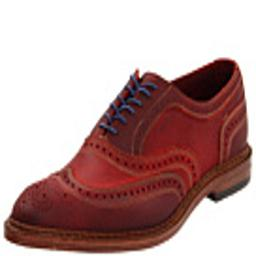}\vspace{-0.1cm}\caption*{\small{Ref 2}}
    \end{subfigure}
    \begin{subfigure}{1.6cm}
    \includegraphics[trim=0cm 0cm 0cm 0cm,clip=true,width=1.6cm]{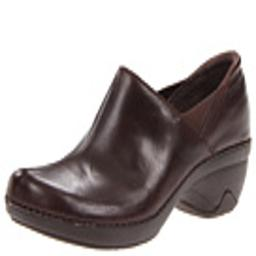}\vspace{-0.1cm}\caption*{\small{Ref 3}}
    \end{subfigure}
    \begin{subfigure}{1.6cm}
    \includegraphics[trim=0cm 0cm 0cm 0cm,clip=true,width=1.6cm]{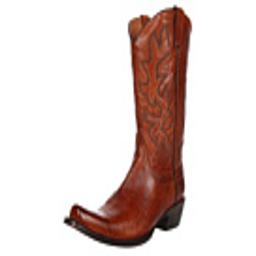}\vspace{-0.1cm}\caption*{\small{Ref 4}}
    \end{subfigure}
    \begin{subfigure}{1.6cm}
    \includegraphics[trim=0cm 0cm 0cm 0cm,clip=true,width=1.6cm]{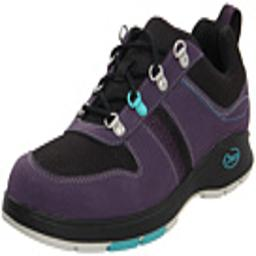}\vspace{-0.1cm}\caption*{\small{Ref 5}}
    \end{subfigure}
    \begin{subfigure}{1.6cm}
    \includegraphics[trim=0cm 0cm 0cm 0cm,clip=true,width=1.6cm]{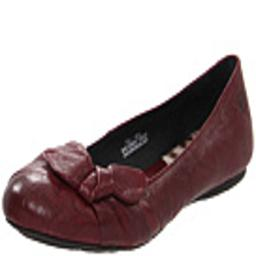}\vspace{-0.1cm}\caption*{\small{Ref 6}}
    \end{subfigure}
    
    \includegraphics[width=1.6cm]{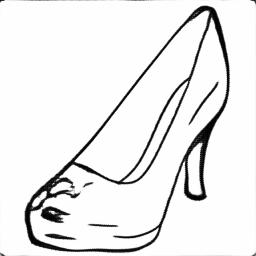}
    \includegraphics[width=1.6cm]{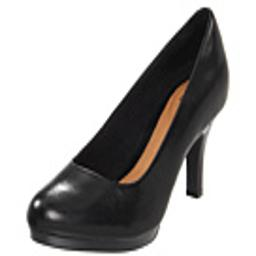}
    \includegraphics[trim=0cm 0cm 0cm 0cm,clip=true,width=1.6cm]{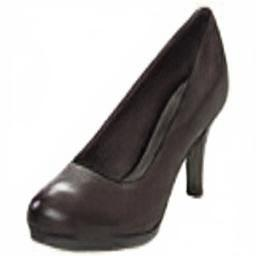}
    \includegraphics[trim=0cm 0cm 0cm 0cm,clip=true,width=1.6cm]{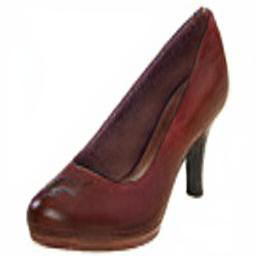}
    \includegraphics[trim=0cm 0cm 0cm 0cm,clip=true,width=1.6cm]{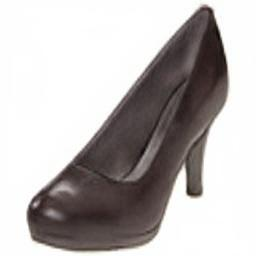}
    \includegraphics[trim=0cm 0cm 0cm 0cm,clip=true,width=1.6cm]{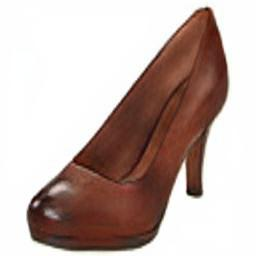}
    \includegraphics[trim=0cm 0cm 0cm 0cm,clip=true,width=1.6cm]{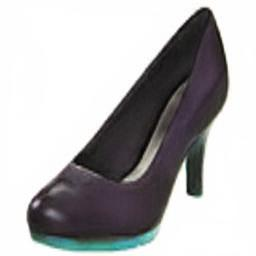}
    \includegraphics[trim=0cm 0cm 0cm 0cm,clip=true,width=1.6cm]{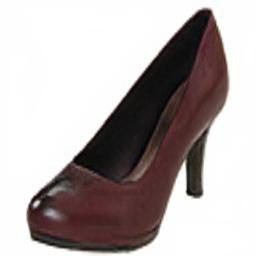}
    
    \begin{subfigure}{1.6cm}
    \includegraphics[trim=0cm 0cm 0cm 0cm,clip=true,width=1.6cm]{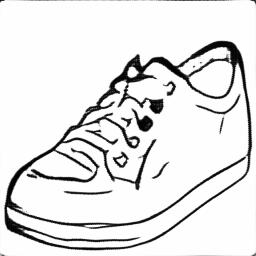}\vspace{-0.1cm}\caption*{\small{Input}}
    \end{subfigure}
    \begin{subfigure}{1.6cm}
    \includegraphics[trim=0cm 0cm 0cm 0cm,clip=true,width=1.6cm]{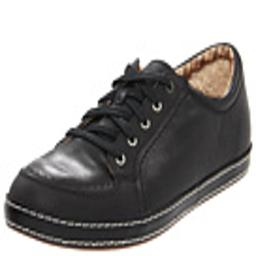}\vspace{-0.1cm}\caption*{\small{GT}}
    \end{subfigure}
    \begin{subfigure}{1.6cm}
    \includegraphics[trim=0cm 0cm 0cm 0cm,clip=true,width=1.6cm]{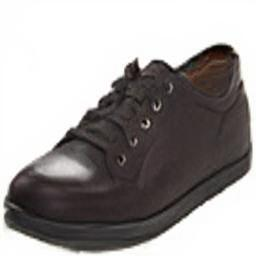}\vspace{-0.1cm}\caption*{\small{Result 1}}
    \end{subfigure}
    \begin{subfigure}{1.6cm}
    \includegraphics[trim=0cm 0cm 0cm 0cm,clip=true,width=1.6cm]{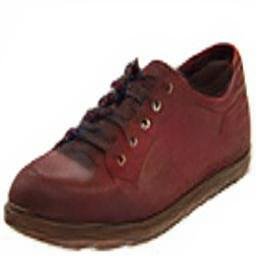}\vspace{-0.1cm}\caption*{\small{Result 2}}
    \end{subfigure}
    \begin{subfigure}{1.6cm}
    \includegraphics[trim=0cm 0cm 0cm 0cm,clip=true,width=1.6cm]{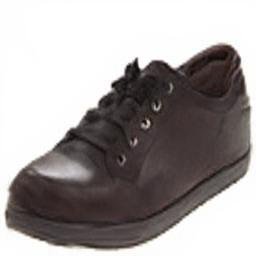}\vspace{-0.1cm}\caption*{\small{Result 3}}
    \end{subfigure}
    \begin{subfigure}{1.6cm}
    \includegraphics[trim=0cm 0cm 0cm 0cm,clip=true,width=1.6cm]{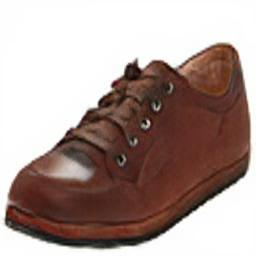}\vspace{-0.1cm}\caption*{\small{Result 4}}
    \end{subfigure}
    \begin{subfigure}{1.6cm}
    \includegraphics[trim=0cm 0cm 0cm 0cm,clip=true,width=1.6cm]{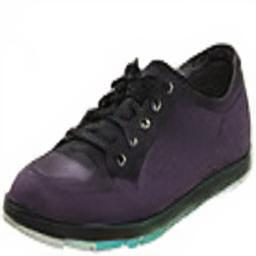}\vspace{-0.1cm}\caption*{\small{Result 5}}
    \end{subfigure}
    \begin{subfigure}{1.6cm}
    \includegraphics[trim=0cm 0cm 0cm 0cm,clip=true,width=1.6cm]{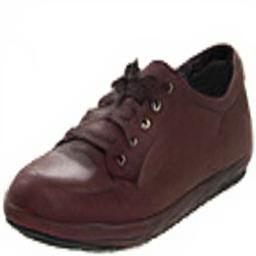}\vspace{-0.1cm}\caption*{\small{Result 6}}
    \end{subfigure}
    \caption{Results in shoe dataset with the refined sketches}
    \label{fig:moreshoes}
\end{figure}

\begin{figure}[!ht]
    \centering
    \captionsetup{size=small}
    \includegraphics[width=1.6cm]{fig/white.png}
    \includegraphics[width=1.6cm]{fig/white.png}
    \begin{subfigure}{1.6cm}
    \includegraphics[trim=0cm 0cm 0cm 0cm,clip=true,width=1.6cm]{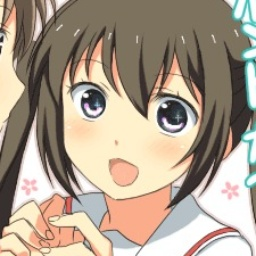}\vspace{-0.1cm}\caption*{\small{Ref 1}}
    \end{subfigure}
    \begin{subfigure}{1.6cm}
    \includegraphics[trim=0cm 0cm 0cm 0cm,clip=true,width=1.6cm]{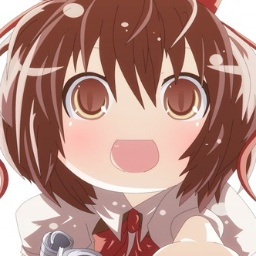}\vspace{-0.1cm}\caption*{\small{Ref 2}}
    \end{subfigure}
    \begin{subfigure}{1.6cm}
    \includegraphics[trim=0cm 0cm 0cm 0cm,clip=true,width=1.6cm]{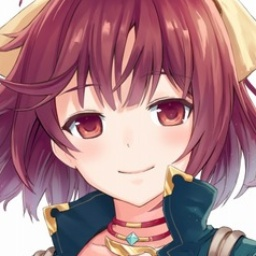}\vspace{-0.1cm}\caption*{\small{Ref 3}}
    \end{subfigure}
    \begin{subfigure}{1.6cm}
    \includegraphics[trim=0cm 0cm 0cm 0cm,clip=true,width=1.6cm]{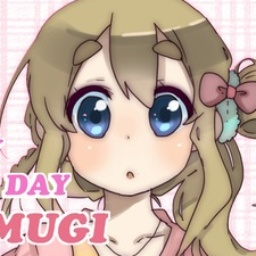}\vspace{-0.1cm}\caption*{\small{Ref 4}}
    \end{subfigure}
    \begin{subfigure}{1.6cm}
    \includegraphics[trim=0cm 0cm 0cm 0cm,clip=true,width=1.6cm]{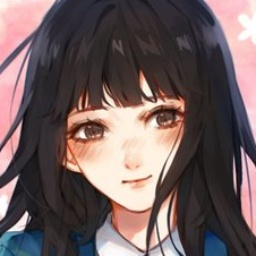}\vspace{-0.1cm}\caption*{\small{Ref 5}}
    \end{subfigure}
    \begin{subfigure}{1.6cm}
    \includegraphics[trim=0cm 0cm 0cm 0cm,clip=true,width=1.6cm]{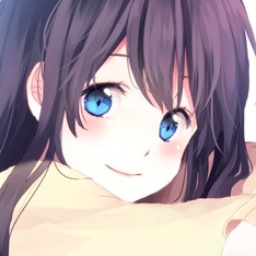}\vspace{-0.1cm}\caption*{\small{Ref 6}}
    \end{subfigure}

    \begin{subfigure}{1.6cm}
    \includegraphics[trim=0cm 0cm 0cm 0cm,clip=true,width=1.6cm]{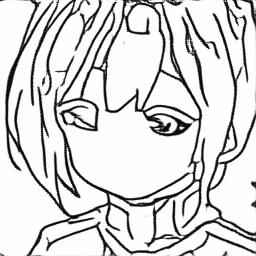}\vspace{-0.1cm}\caption*{\small{Input}}
    \end{subfigure}
    \begin{subfigure}{1.6cm}
    \includegraphics[trim=0cm 0cm 0cm 0cm,clip=true,width=1.6cm]{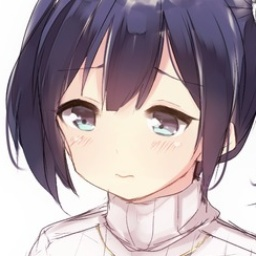}\vspace{-0.1cm}\caption*{\small{GT}} 
    \end{subfigure}
    \begin{subfigure}{1.6cm}
    \includegraphics[trim=0cm 0cm 0cm 0cm,clip=true,width=1.6cm]{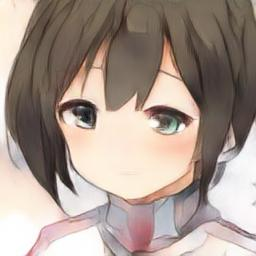}\vspace{-0.1cm}\caption*{\small{Result 1}}
    \end{subfigure}
    \begin{subfigure}{1.6cm}
    \includegraphics[trim=0cm 0cm 0cm 0cm,clip=true,width=1.6cm]{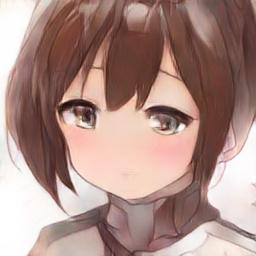}\vspace{-0.1cm}\caption*{\small{Result 2}}
    \end{subfigure}
    \begin{subfigure}{1.6cm}
    \includegraphics[trim=0cm 0cm 0cm 0cm,clip=true,width=1.6cm]{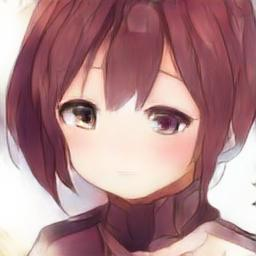}\vspace{-0.1cm}\caption*{\small{Result 3}}
    \end{subfigure}
    \begin{subfigure}{1.6cm}
    \includegraphics[trim=0cm 0cm 0cm 0cm,clip=true,width=1.6cm]{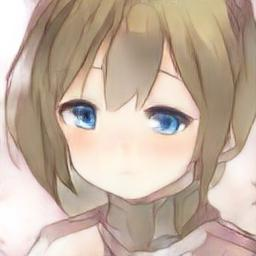}\vspace{-0.1cm}\caption*{\small{Result 4}}
    \end{subfigure}
    \begin{subfigure}{1.6cm}
    \includegraphics[trim=0cm 0cm 0cm 0cm,clip=true,width=1.6cm]{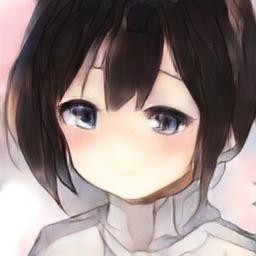}\vspace{-0.1cm}\caption*{\small{Result 5}}
    \end{subfigure}
    \begin{subfigure}{1.6cm}
    \includegraphics[trim=0cm 0cm 0cm 0cm,clip=true,width=1.6cm]{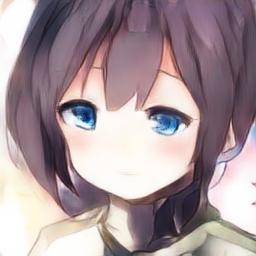}\vspace{-0.1cm}\caption*{\small{Result 6}}
    \end{subfigure}

   \includegraphics[width=1.6cm]{fig/white.png}
    \includegraphics[width=1.6cm]{fig/white.png}
    \begin{subfigure}{1.6cm}
    \includegraphics[trim=0cm 0cm 0cm 0cm,clip=true,width=1.6cm]{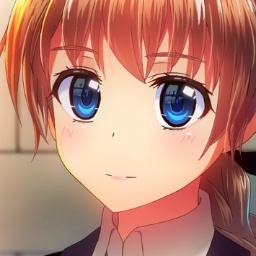}\vspace{-0.1cm}\caption*{\small{Ref 7}}
    \end{subfigure}
    \begin{subfigure}{1.6cm}
    \includegraphics[trim=0cm 0cm 0cm 0cm,clip=true,width=1.6cm]{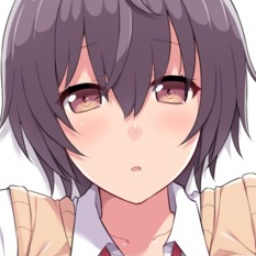}\vspace{-0.1cm}\caption*{\small{Ref 8}}
    \end{subfigure}
    \begin{subfigure}{1.6cm}
    \includegraphics[trim=0cm 0cm 0cm 0cm,clip=true,width=1.6cm]{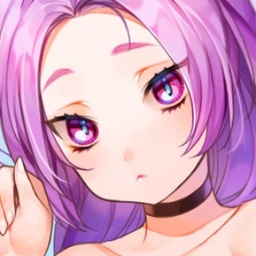}\vspace{-0.1cm}\caption*{\small{Ref 9}}
    \end{subfigure}
    \begin{subfigure}{1.6cm}
    \includegraphics[trim=0cm 0cm 0cm 0cm,clip=true,width=1.6cm]{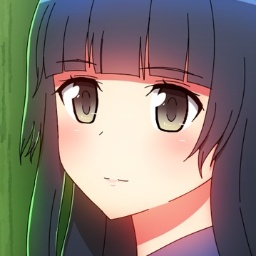}\vspace{-0.1cm}\caption*{\small{Ref 10}}
    \end{subfigure}
    \begin{subfigure}{1.6cm}
    \includegraphics[trim=0cm 0cm 0cm 0cm,clip=true,width=1.6cm]{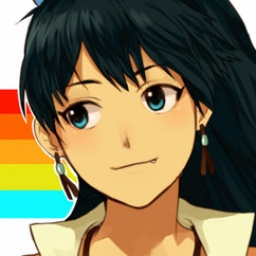}\vspace{-0.1cm}\caption*{\small{Ref 11}}
    \end{subfigure}
    \begin{subfigure}{1.6cm}
    \includegraphics[trim=0cm 0cm 0cm 0cm,clip=true,width=1.6cm]{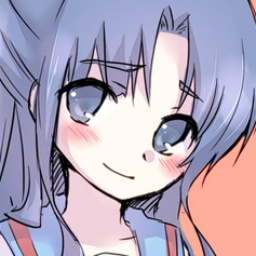}\vspace{-0.1cm}\caption*{\small{Ref 12}}
    \end{subfigure}

    \begin{subfigure}{1.6cm}
    \includegraphics[trim=0cm 0cm 0cm 0cm,clip=true,width=1.6cm]{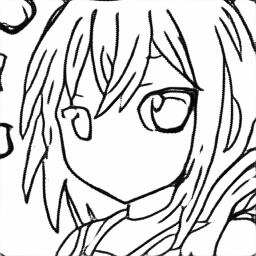}\vspace{-0.1cm}\caption*{\small{Input}}
    \end{subfigure}
    \begin{subfigure}{1.6cm}
    \includegraphics[trim=0cm 0cm 0cm 0cm,clip=true,width=1.6cm]{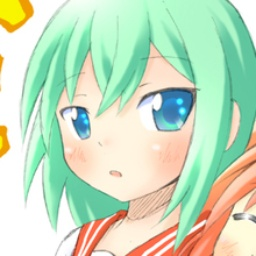}\vspace{-0.1cm}\caption*{\small{GT}} 
    \end{subfigure}
    \begin{subfigure}{1.6cm}
    \includegraphics[trim=0cm 0cm 0cm 0cm,clip=true,width=1.6cm]{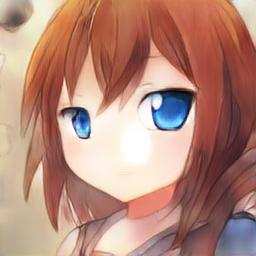}\vspace{-0.1cm}\caption*{\small{Result 1}}
    \end{subfigure}
    \begin{subfigure}{1.6cm}
    \includegraphics[trim=0cm 0cm 0cm 0cm,clip=true,width=1.6cm]{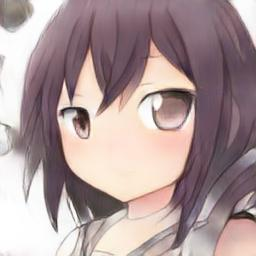}\vspace{-0.1cm}\caption*{\small{Result 2}}
    \end{subfigure}
    \begin{subfigure}{1.6cm}
    \includegraphics[trim=0cm 0cm 0cm 0cm,clip=true,width=1.6cm]{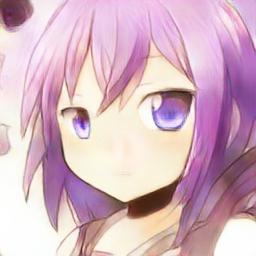}\vspace{-0.1cm}\caption*{\small{Result 3}}
    \end{subfigure}
    \begin{subfigure}{1.6cm}
    \includegraphics[trim=0cm 0cm 0cm 0cm,clip=true,width=1.6cm]{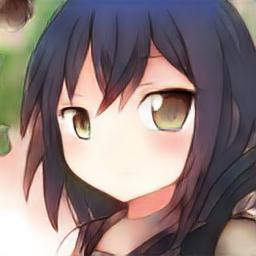}\vspace{-0.1cm}\caption*{\small{Result 4}}
    \end{subfigure}
    \begin{subfigure}{1.6cm}
    \includegraphics[trim=0cm 0cm 0cm 0cm,clip=true,width=1.6cm]{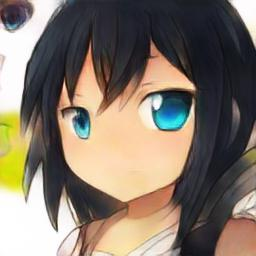}\vspace{-0.1cm}\caption*{\small{Result 5}}
    \end{subfigure}
    \begin{subfigure}{1.6cm}
    \includegraphics[trim=0cm 0cm 0cm 0cm,clip=true,width=1.6cm]{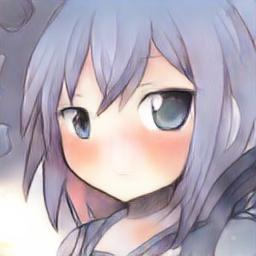}\vspace{-0.1cm}\caption*{\small{Result 6}}
    \end{subfigure}
   
\label{fig:more_anime}
\caption{\small{More Results on the Danbooru\cite{danbooru2018} dataset}}
\end{figure}

\begin{figure}[!ht]
    \centering
    \begin{subfigure}{3cm}
    \includegraphics[width=3cm]{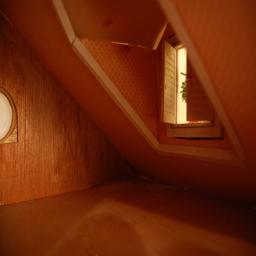}\caption{Ref}
    \end{subfigure}
    \begin{subfigure}{3cm}
    \includegraphics[width=3cm]{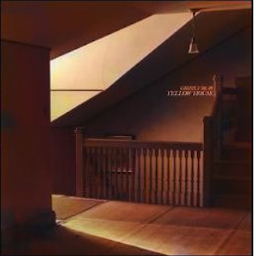}\caption{Result}
    \end{subfigure}
    \begin{subfigure}{3cm}
    \includegraphics[width=3cm]{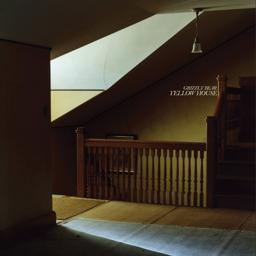}\caption{GT}
    \end{subfigure}
    \caption{\small{Failure case: if the semantic relationship between the input and the reference is inadequate, the semantic guided I2I will be degraded to a global style control.}}
    \label{fig:my_label}
\end{figure}
